# Supplementary material for: Ornstein-Uhlenbeck Adaptation as a Mechanism for Learning in Brains and Machines
Source: arXiv:2410.13563 source file (2024-12-09)
Supplement: Supplementary file 1 [file appendices.tex]

\section{Hyper-parameters interaction}

\begin{figure}[!ht]
\centering
\includegraphics[width=\textwidth]{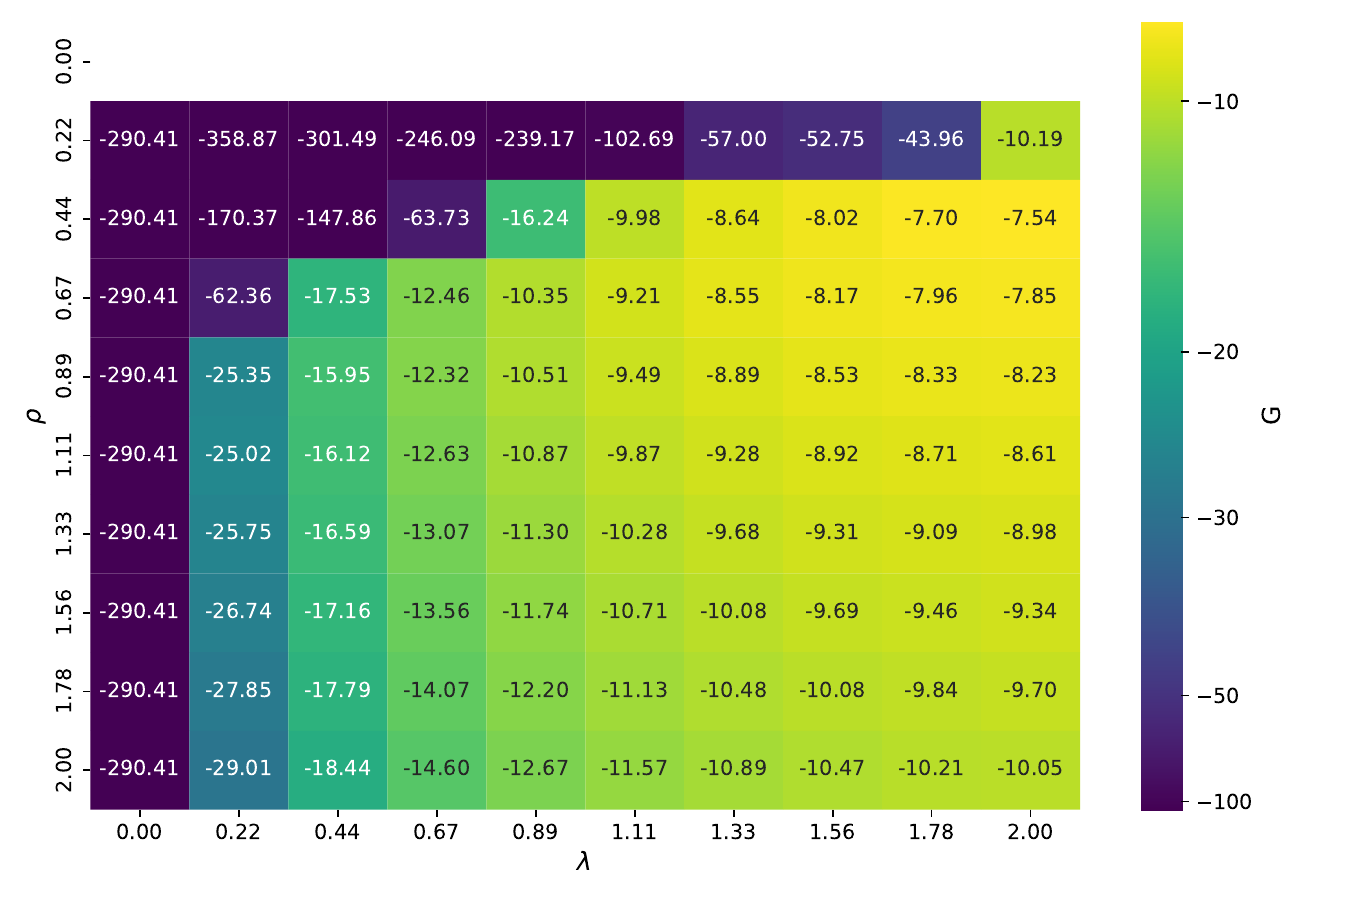}
\caption{Blabla.}
\label{fig:grid_search}
\end{figure}
